# Supplementary material for: Stability Bounds for Learning-Based Adaptive Control of Discrete-Time Multi-Dimensional Stochastic Linear Systems with Input Constraints
Source: arXiv:2304.00569 source file (2023-04-02)
Supplement: Supplementary file 1 [file 07-appendix.tex]

% \begin{assumption} \label{assump:large-sat-level}
%     The saturation level $D$ satisfies $D > 2 \Vert  \mathcal{R}^{\dagger} \Vert \log{( \mathbb{E} [e^{ |\bar{V}_0 + \bar{W}_0| }] )}$.
% \end{assumption}

% \begin{lemma}
%     Suppose Assumptions \ref{assump:disturbance}, \ref{assump:reachable}, \ref{assump:exciting-noise}, and \ref{assump:bmsb} hold. For all $\epsilon > 0$, there exist $L_1 > 0$ and a function $L_2 : \mathbb{R}^n \rightarrow  \mathbb{R}_{>0}$ such that
%     \begin{align}
%         K(\epsilon,\delta) \leq L_2(x_0)(1/\delta)^{L_1}
%     \end{align}
%     holds for all $x_0 \in \mathbb{R}^n$.
% \end{lemma}
